# Supplementary material for: Maximum likelihood estimation for a stochastic SEIR system for COVID-19
Source: arXiv:2111.14261 source file (2021-11-24)
Supplement: Supplementary file 1 [file appendix_A.tex]

From {\color{blue} (4)} and {\color{blue} (5)} we get the following two expressions for the noise $dW(t)$
\begin{align}
 dW(t)&= -\frac{1}{\sigma}d\big(\log (1-S_t) \big)  -\Big[  \frac{\mu}{\sigma } -\frac{f_\beta  S}{\sigma (1-S)} + \frac{\gamma  R}{\sigma (1-S)} + \tfrac{1}{2} \sigma \Big] dt \label{dlogS1}\\
 dW(t) &= -\frac{1}{\sigma} d(\log (E_t)) - \Big[ -\frac{f_\beta  S  }{\sigma E} + \frac{  \kappa   }{\sigma }  + \frac{\mu }{\sigma }  +  \frac{1}{2} \sigma\Big] dt. \label{dlogE1}
 \end{align}

We use the last expressions to study the first term in the right side of {\color{blue} (10)}.
First, we rewrite {\color{blue} (10)} as:

\begin{align}
\label{MLE-beta-beta1}
\begin{pmatrix}
\hat{\beta_s}  - \beta_{s,0} \\
\hat{\beta_a} - \beta_{a,0} 
\end{pmatrix}
&=
- \sigma \frac{1}{J_s J_a - J_{sa}^2}\begin{pmatrix}
J_a(T) & -J_{sa}(T)\\
-J_{sa}(T & J_s(T)
\end{pmatrix} \,    \begin{pmatrix} \int_0^T \Big[ \frac{S(t) I_s(t)}{ (1-S(t))} +  \frac{S(t) I_s(t)}{ E(t)} \Big]  dW(t) \\
\int_0^T \Big[ \frac{S(t) I_a(t)}{ (1-S(t))} +  \frac{S(t) I_a(t)}{ E(t)} \Big]  dW(t)
\end{pmatrix}\nonumber\\
& \hspace*{-1cm} =
- \frac{\sigma }{J_s J_a - J_{sa}^2} \,    \begin{pmatrix} J_a(T) \int_0^T \Big[ \frac{S(t) I_s(t)}{ (1-S(t))} + \frac{S(t) I_s(t)}{ E(t)} \Big]  dW(t) - J_{sa}(T) \int_0^T \Big[ \frac{S(t) I_a(t)}{ (1-S(t))} + \frac{S(t) I_a(t)}{ E(t)} \Big]  dW(t) \\
-J_{sa}(T) \int_0^T \Big[ \frac{S(t) I_s(t)}{ (1-S(t))} + \frac{S(t) I_s(t)}{ E(t)} \Big]  dW(t) + J_{s}(T) \int_0^T \Big[ \frac{S(t) I_a(t)}{ (1-S(t))} + \frac{S(t) I_a(t)}{ E(t)} \Big]  dW(t)
\end{pmatrix}    
\end{align}    
  
 We focus on the two stochastic integrals in the last expressions and use  \eqref{dlogS1} and \eqref{dlogE1}. Thus,
    
\begin{align}
  - \sigma & \int_0^T \Big[ \frac{S(t) I_s(t)}{ (1-S(t))} +  \frac{S(t) I_s(t)}{ E(t)} \Big]  dW(t)\nonumber\\
&=  - \sigma  \int_0^T  \frac{S(t) I_s(t)}{ (1-S(t))} \Big[ -\frac{1}{\sigma}d\big(\log (1-S_t) \big)\Big] \nonumber\\
&\quad - \sigma  \int_0^T  \frac{S(t) I_s(t)}{ (1-S(t))} \Big[ -\Big(  \frac{\mu}{\sigma } -\frac{ f_{\beta_0}  S }{\sigma (1-S)} + \frac{\gamma  R}{\sigma (1-S)} + \tfrac{1}{2} \sigma \Big) dt \Big]\nonumber \\
&- \, \sigma  \int_0^T   \frac{S(t) I_s(t)}{ E(t)} \Big[ -\frac{1}{\sigma} d(\log (E_t)) - \Big( -\frac{ f_{\beta_0}  S }{\sigma E} + \frac{  \kappa   }{\sigma }  + \frac{\mu }{\sigma }  +  \frac{1}{2} \sigma\Big) dt \Big]\nonumber\\
&=  -   \int_0^T  \frac{S(t) I_s(t)}{ (1-S(t))} \Big[ -d\big(\log (1-S_t) \big)\Big] \nonumber\\
&\, -   \int_0^T  \frac{S(t) I_s(t)}{ (1-S(t))} \Big[ -\Big(  \mu + \frac{\gamma  R}{ (1-S)} + \tfrac{1}{2} \sigma^2 \Big) dt \Big] - J_s(T)  \beta_{s,0} - J_{sa}(T) \beta_{a,0} \nonumber \\
&- \,   \int_0^T   \frac{S(t) I_s(t)}{ E(t)} \Big[ -  d(\log (E_t)) - \Big(   \mu   +  \frac{1}{2} \sigma^2 \Big) dt \Big] +  \,   \kappa    \int_0^T   \frac{S(t) I_s(t)}{ E(t)} dt, \nonumber
\end{align}

For the second stochastic integral in the right side of  \eqref{MLE-beta-beta1}

\begin{align}
  - \sigma & \int_0^T \Big[ \frac{S(t) I_a(t)}{ (1-S(t))} +  \frac{S(t) I_a(t)}{ E(t)} \Big]  dW(t)\nonumber\\
&=  - \sigma  \int_0^T  \frac{S(t) I_a(t)}{ (1-S(t))} \Big[ -\frac{1}{\sigma}d\big(\log (1-S_t) \big)\Big] \nonumber\\
&\quad - \sigma  \int_0^T  \frac{S(t) I_a(t)}{ (1-S(t))} \Big[ -\Big(  \frac{\mu}{\sigma } -\frac{ f_{\beta_0}  S }{\sigma (1-S)} + \frac{\gamma  R}{\sigma (1-S)} + \tfrac{1}{2} \sigma \Big) dt \Big]\nonumber \\
&- \, \sigma  \int_0^T   \frac{S(t) I_a(t)}{ E(t)} \Big[ -\frac{1}{\sigma} d(\log (E_t)) - \Big( -\frac{ f_{\beta_0}  S }{\sigma E} + \frac{  \kappa   }{\sigma }  + \frac{\mu }{\sigma }  +  \frac{1}{2} \sigma\Big) dt \Big]\nonumber\\
&=  -   \int_0^T  \frac{S(t) I_a(t)}{ (1-S(t))} \Big[ -d\big(\log (1-S_t) \big)\Big] \nonumber\\
&\, -   \int_0^T  \frac{S(t) I_a(t)}{ (1-S(t))} \Big[ -\Big(  \mu + \frac{\gamma  R}{ (1-S)} + \tfrac{1}{2} \sigma^2 \Big) dt \Big] - J_{sa}(T)  \beta_{s,0} - J_a(T) \beta_{a,0}  \nonumber \\
&- \,   \int_0^T   \frac{S(t) I_a(t)}{ E(t)} \Big[ -  d(\log (E_t)) - \Big(   \mu   +  \frac{1}{2} \sigma^2 \Big) dt \Big] +  \,   \kappa    \int_0^T   \frac{S(t) I_a(t)}{ E(t)} dt. \nonumber
\end{align}

Then, 

\begin{align*}
 \hat{\beta_s} & - \beta_{s,0} \\
 & = - \frac{\sigma }{J_s J_a - J_{sa}^2} \left[ J_a(T) \int_0^T \Big[ \frac{S(t) I_s(t)}{ (1-S(t))} + \frac{S(t) I_s(t)}{ E(t)} \Big]  dW(t) - J_{sa}(T) \int_0^T \Big[ \frac{S(t) I_a(t)}{ (1-S(t))} + \frac{S(t) I_a(t)}{ E(t)} \Big]  dW(t) \right] \\
 &=  \frac{1 }{J_s J_a - J_{sa}^2} \Bigg[  -  J_a(T) \int_0^T  \frac{S(t) I_s(t)}{ (1-S(t))} \Big[ -d\big(\log (1-S_t) \big)\Big] \nonumber\\
&\, -   J_a(T) \int_0^T  \frac{S(t) I_s(t)}{ (1-S(t))} \Big[ -\Big(  \mu + \frac{\gamma  R}{ (1-S)} + \tfrac{1}{2} \sigma^2 \Big) dt \Big] - J_a(T)  J_s(T)  \beta_{s,0} - J_a(T)  J_{sa}(T) \beta_{a,0} \nonumber \\
&- \,   J_a(T) \int_0^T   \frac{S(t) I_s(t)}{ E(t)} \Big[ -  d(\log (E_t)) - \Big(   \mu   +  \frac{1}{2} \sigma^2 \Big) dt \Big] +  \,   \kappa    J_a(T) \int_0^T   \frac{S(t) I_s(t)}{ E(t)} dt\\
&\,+  J_{sa}(T) \int_0^T   \frac{S(t) I_a(t)}{ (1-S(t))} \Big[ -d\big(\log (1-S_t) \big)\Big] \nonumber\\
&\, +    J_{sa}(T) \int_0^T  \frac{S(t) I_a(t)}{ (1-S(t))} \Big[ -\Big(  \mu + \frac{\gamma  R}{ (1-S)} + \tfrac{1}{2} \sigma^2 \Big) dt \Big] + J_{sa}^2(T)  \beta_{s,0} +  J_{sa}(T) J_a(T) \beta_{a,0}  \nonumber \\
& \, +   J_{sa}(T) \int_0^T   \frac{S(t) I_a(t)}{ E(t)} \Big[ -  d(\log (E_t)) - \Big(   \mu   +  \frac{1}{2} \sigma^2 \Big) dt \Big] -  \,     \kappa  J_{sa}(T)   \int_0^T   \frac{S(t) I_a(t)}{ E(t)} dt\Bigg].
\end{align*}

which implies {\color{blue} (17)}. \\

Similarly,

\begin{align*}
 \hat{\beta_a} & - \beta_{a,0} \\
 & = - \frac{\sigma }{J_s J_a - J_{sa}^2} \left[ -J_{sa}(T) \int_0^T \Big[ \frac{S(t) I_s(t)}{ (1-S(t))} + \frac{S(t) I_s(t)}{ E(t)} \Big]  dW(t) + J_{s}(T) \int_0^T \Big[ \frac{S(t) I_a(t)}{ (1-S(t))} + \frac{S(t) I_a(t)}{ E(t)} \Big]  dW(t) \right] \\
 &=  \frac{1 }{J_s J_a - J_{sa}^2} \Bigg[   J_{sa}(T) \int_0^T  \frac{S(t) I_s(t)}{ (1-S(t))} \Big[ -d\big(\log (1-S_t) \big)\Big] \nonumber\\
&\, +  J_{sa}(T) \int_0^T  \frac{S(t) I_s(t)}{ (1-S(t))} \Big[ -\Big(  \mu + \frac{\gamma  R}{ (1-S)} + \tfrac{1}{2} \sigma^2 \Big) dt \Big] + J_{sa}(T)  J_s(T)  \beta_{s,0} + J_{sa}(T)  J_{sa}(T) \beta_{a,0} \nonumber \\
& \, +  J_{sa}(T) \int_0^T   \frac{S(t) I_s(t)}{ E(t)} \Big[ -  d(\log (E_t)) - \Big(   \mu   +  \frac{1}{2} \sigma^2 \Big) dt \Big] -  \,   \kappa    J_{sa}(T) \int_0^T   \frac{S(t) I_s(t)}{ E(t)} dt\\
&\,- J_{s}(T) \int_0^T   \frac{S(t) I_a(t)}{ (1-S(t))} \Big[ -d\big(\log (1-S_t) \big)\Big] \nonumber\\
&\, -    J_{s}(T) \int_0^T  \frac{S(t) I_a(t)}{ (1-S(t))} \Big[ -\Big(  \mu + \frac{\gamma  R}{ (1-S)} + \tfrac{1}{2} \sigma^2 \Big) dt \Big] - J_s(T)  J_{sa}  \beta_{s,0} -  J_{s}(T) J_a(T) \beta_{a,0}  \nonumber \\
& \, -   J_{s}(T) \int_0^T   \frac{S(t) I_a(t)}{ E(t)} \Big[ -  d(\log (E_t)) - \Big(   \mu   +  \frac{1}{2} \sigma^2 \Big) dt \Big]  \,    + \kappa  J_{s}(T)   \int_0^T   \frac{S(t) I_a(t)}{ E(t)} dt\Bigg].
\end{align*}

and this implies {\color{blue} (18)}.

To show {\color{blue} (19)}, we proceed as before, but now we use the SDEs {\color{blue} (7)}, {\color{blue} (8)} and the integral version of {\color{blue} (5)}, this allow us to write the noise $dW(t)$ and $W(T)$ in a convenient expression for the calculations. Indeed, we have,

\begin{align*}
(p-  p_0 )J_2(T) &= \sigma \int_0^T \Big[  -\frac{\kappa E(t)}{ I_a(t)} +
\frac{\kappa E(t)}{ I_s(t)} \Big] dW(t)
 \end{align*} 
At this point for the first term in the last equality we will use the SDE {\color{blue} (6)} and for the second the SDE {\color{blue} (7)}, then
\begin{align*}
(p-  p_0 )J_2(T) 
 &= -\sigma \int_0^T \frac{\kappa E(t)}{ I_a(t)} dW(t) + \sigma \int_0^T 
\frac{\kappa E(t)}{ I_s(t)}  dW(t) \\
&= -\sigma \int_0^T  \frac{\kappa E(t)}{ I_a(t)} \Big[ -\frac{1}{\sigma} d(\log (I_a)) -   \Big( -\frac{\kappa  p_0 E}{\sigma I_a} +\frac{(\alpha_a + \mu )}{\sigma }  +  \frac{1}{2} \sigma\Big) dt  \Big]\\
&\, +   \sigma \int_0^T  \frac{\kappa E(t)}{ I_s(t)} \Big[-\frac{1}{\sigma} d(\log (I_s))  - \Big( -\frac{\kappa (1-p_0) E}{\sigma I_s} + \frac{(\alpha_s + \mu )}{\sigma } +  \frac{1}{2} \sigma\Big) dt \Big]
\\
&=  \int_0^T  \frac{\kappa E(t)}{ I_a(t)}\Big[ d(\log (I_a))  + \Big(  (\alpha_a + \mu ) +  \frac{1}{2} \sigma^2\Big) dt \Big] -  p_0  \int_0^T  \frac{\kappa^2 E^2(t)}{ I_a^2(t)} dt \\
&\, +    \int_0^T  \frac{\kappa E(t)}{ I_s(t)} \Big[ - d(\log (I_s)) +\frac{\kappa E}{ I_s}  -   \Big( (\alpha_s + \mu )  +  \frac{1}{2} \sigma^2\Big) dt  \Big]  -  p_0  \int_0^T  \frac{\kappa^2 E^2(t)}{ I_s^2(t)} dt \\
&=  \int_0^T  \frac{\kappa E(t)}{ I_a(t)}\Big[ d(\log (I_a))  + \Big(  (\alpha_a + \mu ) +  \frac{1}{2} \sigma^2\Big) dt \Big]  \\
&\, +    \int_0^T  \frac{\kappa E(t)}{ I_s(t)} \Big[ - d(\log (I_s)) +\frac{\kappa E}{ I_s}  -   \Big( (\alpha_s + \mu )  +  \frac{1}{2} \sigma^2\Big) dt  \Big]  -  p_0 J_2(T), 
 \end{align*}  
which implies {\color{blue} (19)}.
